# Supplementary material for: Generalized Pairing Wave Functions and Nodal Properties for Electronic Structure Quantum Monte Carlo
Source: arXiv:0712.3066 source file (2007-12-18)
Supplement: Supplementary file 1 [file Backflow_appendix.tex]

\chapter{Value, Gradient and Laplacian of Back-Flow Wave Function}
