# Supplementary material for: Generalized Pairing Wave Functions and Nodal Properties for Electronic Structure Quantum Monte Carlo
Source: arXiv:0712.3066 source file (2007-12-18)
Supplement: Supplementary file 4 [file determinant_analytic_ders.tex]

\chapter{Analytic Derivatives of Determinantal Wave Function  
with Respect to Variational Parameters}
