# Supplementary material for: Generalized Pairing Wave Functions and Nodal Properties for Electronic Structure Quantum Monte Carlo
Source: arXiv:0712.3066 source file (2007-12-18)
Supplement: Supplementary file 5 [file pfaffian_analytic_ders.tex]

\chapter{Analytic Derivatives of Pfaffian Pairing Wave Function 
with Respect to Variational Parameters}\label{appendix:pfaffianders}
